# Supplementary material for: Correlations in uniform spanning trees: a fermionic approach
Source: arXiv:2312.14992 source file (2023-12-22)
Supplement: Supplementary file 1 [file appendix.tex]

\section{Proof of Lemmas~\ref{lem:bij_tau} and~\ref{lem:surg_tau}}\label{app:proof_loc_tau}
In this appendix, we provide the proof of some technical results which we need for the proof of Theorem \ref{thm:main_cum3_cont}.

\begin{proof}[Proof of Lemma~\ref{lem:bij_tau}]
The fact that every $\tau$ induces a permutation on $\mcE_{v}\setminus\{\eta(v)\}$ follows from the definition~\eqref{eq:def_omega}.
For the converse, consider a permutation $\omega\in S(\mcE_{v}\setminus\{\eta(v)\})$. Using the fact that $\gamma$ is fixed in our assumptions, we can reconstruct $\tau$ locally, and in turn $\omega^\tau_v$, according to the values of $\gamma$. If $\gamma(v)=1$ then the only $\tau$ which satisfies $\omega_v^\tau=\omega$ in $\mcE_{v}\setminus\{\eta(v)\}$ is $\tau(f)=\omega(f)$. If instead $\gamma(v)=-1$, the only $\tau$ which satisfies $\omega_v^\tau=\omega$ is $\tau(f)=\omega(f)$ for $f\in \mcE_{v}\setminus\{\eta(v)\}$ and $\tau(\eta(v))=\omega(\gamma\eta(v)).$
\end{proof}
See Figure~\ref{fig:lemma47} for an example.
\begin{figure}[ht!]
    \centering
    \includegraphics[scale=.8]{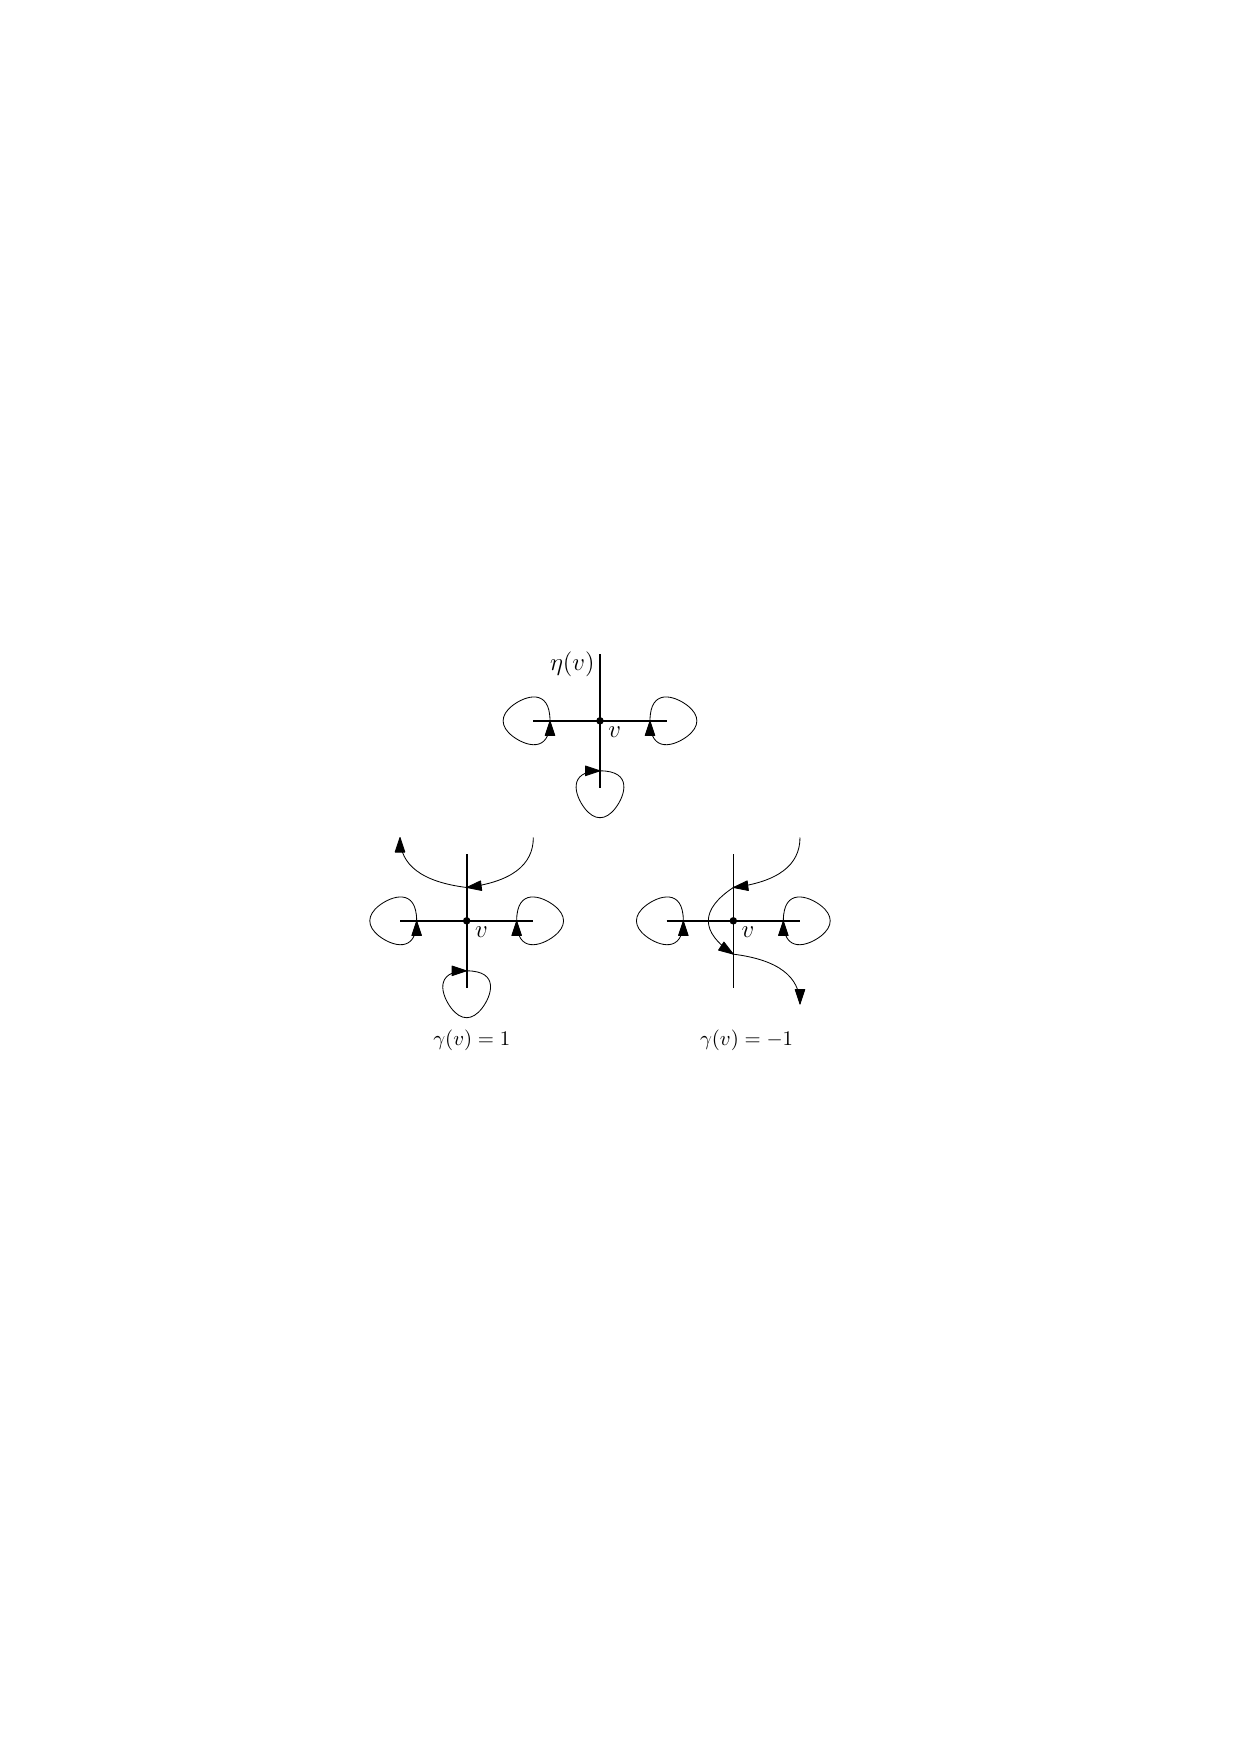}
    \caption{Top: a permutation $\omega\in S(\mcE_{v}\setminus\{\eta(v)\})$. Bottom: there is only one $\tau$ compatible with $\eta,\,\gamma$ that can induce $\omega^\tau_v=\omega$: $\tau$ is depicted on the left if $\gamma(v)=1$ and on the right if $\gamma(v)=-1$).}
    \label{fig:lemma47}
\end{figure}

\begin{proof}[Proof of Lemma~\ref{lem:surg_tau}]
Showing~\eqref{eq:equiv_omega}-\eqref{eq:sgn_tau} is an immediate consequence of Cases~\ref{I} -- \ref{III} (after noticing that $\omega_v^\tau(-\eta(v))=-\eta(v)$ can happen only in Case~\ref{II}), therefore we proceed to proving the three cases under discussion.

\begin{itemize}[wide, labelindent=0pt]
% \begin{itemize}
\item[Case~\ref{I}] Since $\tau$ enters $v$ through $\eta(v)$ and exits immediately through the same edge we can note that $\tau$ is the composition of the two disjoint permutations $\tau\setminus\omega^\tau_v$ and $\omega^\tau_v$. The two conclusions then follow.
\item[Case~\ref{II}] Note that in this case we must have $ \gamma\eta(v)\in \mcE_{v}$ since $\gamma(v)=-1$. 

Let us consider $\prod_{f\in \mcE_{v}\setminus\{-\eta(v)\}}\overline M(f,\,\tau(f)).$ The only term in this product which does not appear in $\prod_{f\in \mcE_{v}\setminus\{\eta(v),\,-\eta(v)\}}\overline M(f,\,\omega^\tau_v(f))$ is $\overline M(\eta(v),\,\tau(\eta(v)))=\overline M(\eta(v),\,-\eta(v))=\overline M(e_1,\,-e_1)$ by~\eqref{eq:def_bar_M}. To justify the expression for $\sign(\tau)$ it is sufficient to notice that $\omega^\tau_v$ does all but one of the transpositions of $\tau$ in $\mcE_{v}\setminus\{\eta(v),\,-\eta(v)\}$, since $-\eta(v)$ is a fixed point for $\omega^\tau_v$.
\item[Case~\ref{III}] Note that, as above, we must have $ \gamma\eta(v)\in \mcE_{v}$. In this case, after $\tau$ enters $v$ through $\eta(v)$, the permutations $\omega^\tau_v$ and $\tau$ are the same until they reach the edge $-\eta(v)$, when $\tau$ departs from $v$ and instead $\omega^\tau_v$ returns to $\tau(\eta(v))$. Therefore
\[
\prod_{f\in \mcE_{v}\setminus  \{-\eta(v)\}} \overline M\left(f,\,\tau(f)\right)=\prod_{f\in \mcE_{v}\setminus  \{\eta(v)\}} \overline M\left(f,\,\omega^\tau_v(f)\right).
\]
Note that, under our assumptions, $\overline M\left(\eta(v),\,\tau(\eta(v))\right)=\overline M\left(-\eta(v),\,\tau(\eta(v))\right)$, so the product over $f\in \mcE_{v}\setminus  \{-\eta(v)\}$ on the left-hand side above transforms into a product over $f\in \mcE_{v}\setminus  \{\eta(v)\}$ on the right-hand side.

Due to the fact that $\omega^\tau_v$ suppresses the jump $-\eta(v) \mapsto \tau(-\eta(v))$ and sets $\omega^\tau_v(-\eta(v))$ equal to $\tau(\eta(v))$, the permutation $\omega^\tau_v$ makes one transposition less than $\tau$ in $\mcE_{v}\setminus\{\eta(v)\}$, justifying $\sign(\tau)=-\sign(\tau\setminus\omega^\tau_v)\sign(\omega_v^\tau)$.
\qedhere
\end{itemize}
\end{proof}
